# Supplementary material for: Mindfulness Meditation and Respiration: Accelerometer-Based Respiration Rate and Mindfulness Progress Estimation to Enhance App Engagement and Mindfulness Skills
Source: arXiv:2507.17688 source file (2025-07-23)
Supplement: Supplementary file 1 [file meta_appendix.tex]

% \section{Revision Notes}
% This document summarizes the actions taken to revise the paper titles \textit{Mindfulness Meditation and Respiration: Accelerometer-Based Respiration Rate and Mindfulness Progress Estimation to Enhance App Engagement and Mindfulness Skills}, which was submitted to IMWUT in February 2025 and received a request for a major revision from the reviewers. This document aims to assist the reviewers in easily finding the changes in the new submission (May 2025) based on the reviews. The document presents the revision information on the new submission along with brief answers to the reviewers' questions. This document consists of four sections, each addressing the concern of one reviewer. In order to keep each section self-contained, some repeated answers are present for the same or similar comments. Major additions to this new submission include Section 7, Section 8.1, Section 9. 

% \input{IMWUT'25/rebuttal/reviewer2}
% \input{IMWUT'25/rebuttal/reviewer1}
% \input{IMWUT'25/rebuttal/reviewer3}
% \input{IMWUT'25/rebuttal/reviewer4}

\section{Code, data and Model availability}
All our codes and models developed in this study can be found in this link.

\href{https://anonymous.4open.science/r/mindfulness-E042/}{https://anonymous.4open.science/r/mindfulness-E042/}

This repository contains the sample dataset, trained models, and the complete pipeline for training and evaluating models for estimating changes in mindfulness skills and respiration rate tracking.

\subsection{Dataset}
Due to agreement with the users, the whole dataset used in this study is not publicly available. A sample of the anonymized dataset is available in the repository to evaluate the model.

\subsection{Respiration Rate Tracking Algorithm}
'respiration rate' folder contains the proposed respiration rate tracking algorithm and the baseline algorithms. 

\subsection{Mindfulness Estimation Model}
All hyperparameters can be found and changed in the 'mindfulness.yaml' file, and the environment can be set up by installing the 'requirements.txt' file.

\parlabel{Saved models} All trained models are stored in the 'saved\_models' folder.

\parlabel{Training pipeline} run 'python main.py' to train the model.

\parlabel{Evaluation pipeline} run 'python evaluate.py' to evaluate the model.
